# Supplementary material for: Out-of-equilibrium Polymorph Selection in Nanoparticle Freezing
Source: arXiv:2009.05316 source file (2020-09-11)
Supplement: Supplementary file 1 [file SupInfo.pdf]

# Supporting Information: Out-of-Equilibrium Polymorph Selection in Nanoparticle Freezing

Jonathan Amodeo,† Fabio Pietrucci,‡ and Julien Lam*,¶

†*Université de Lyon, INSA-Lyon, MATEIS, UMR 5510 CNRS, 69621 Villeurbanne, France*

‡*Sorbonne Université, CNRS UMR 7590, IMPMC, 75005 Paris, France*

¶*Center for Nonlinear Phenomena and Complex Systems, Université Libre de Bruxelles, Code Postal 231, Boulevard du Triomphe, 1050 Brussels, Belgium*

E-mail: julien.lam@ulb.ac.be

## Freezing MD simulations: full dataset

Figures S1, S2 and S3 show all MD freezing simulations performed with a quench duration of about 50, 100 and 200 ns respectively as mentioned in the original article.

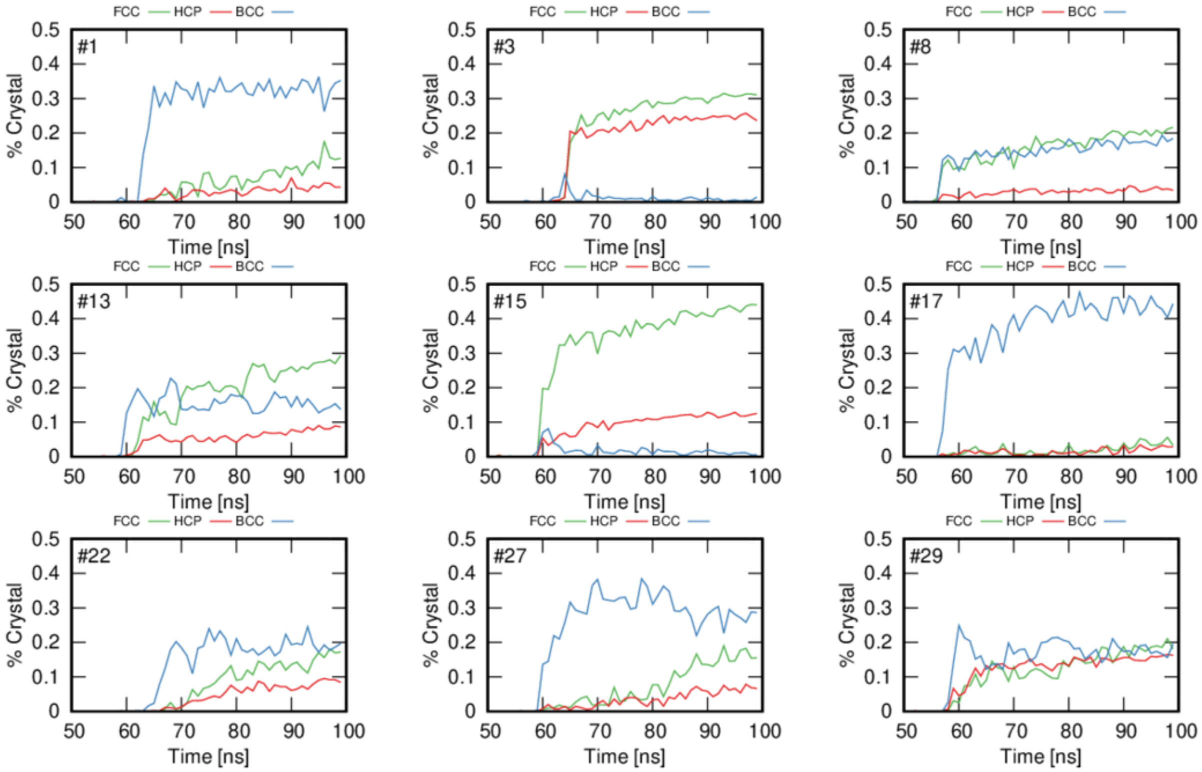


Figure S1: Crystallization kinetics of $Ni_3Al$ nanocrystals at $\tau = 50$ ns.

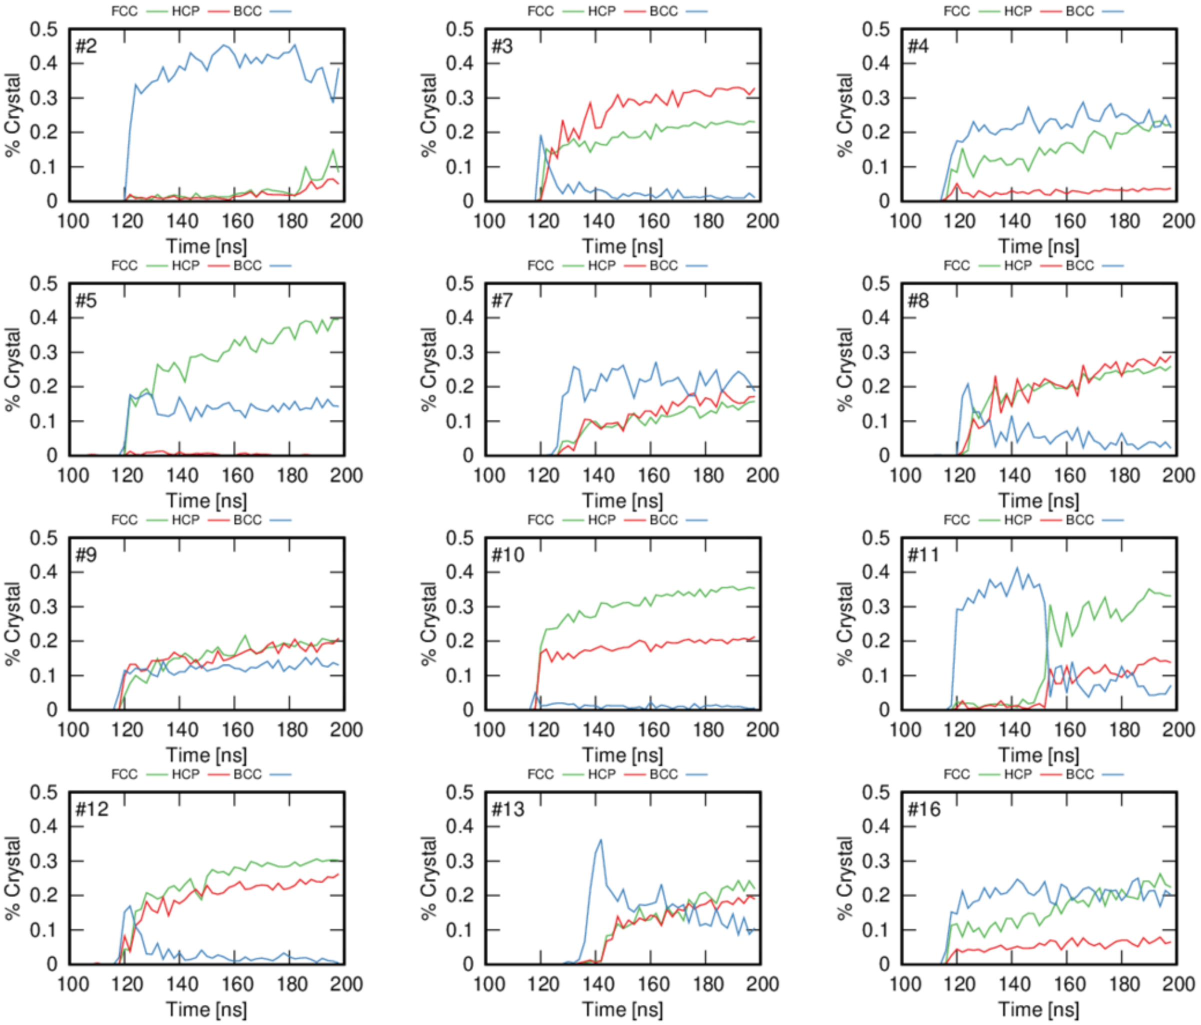


Figure S2: Crystallization kinetics of $Ni_3Al$ nanocrystals at $\tau = 100$ ns.

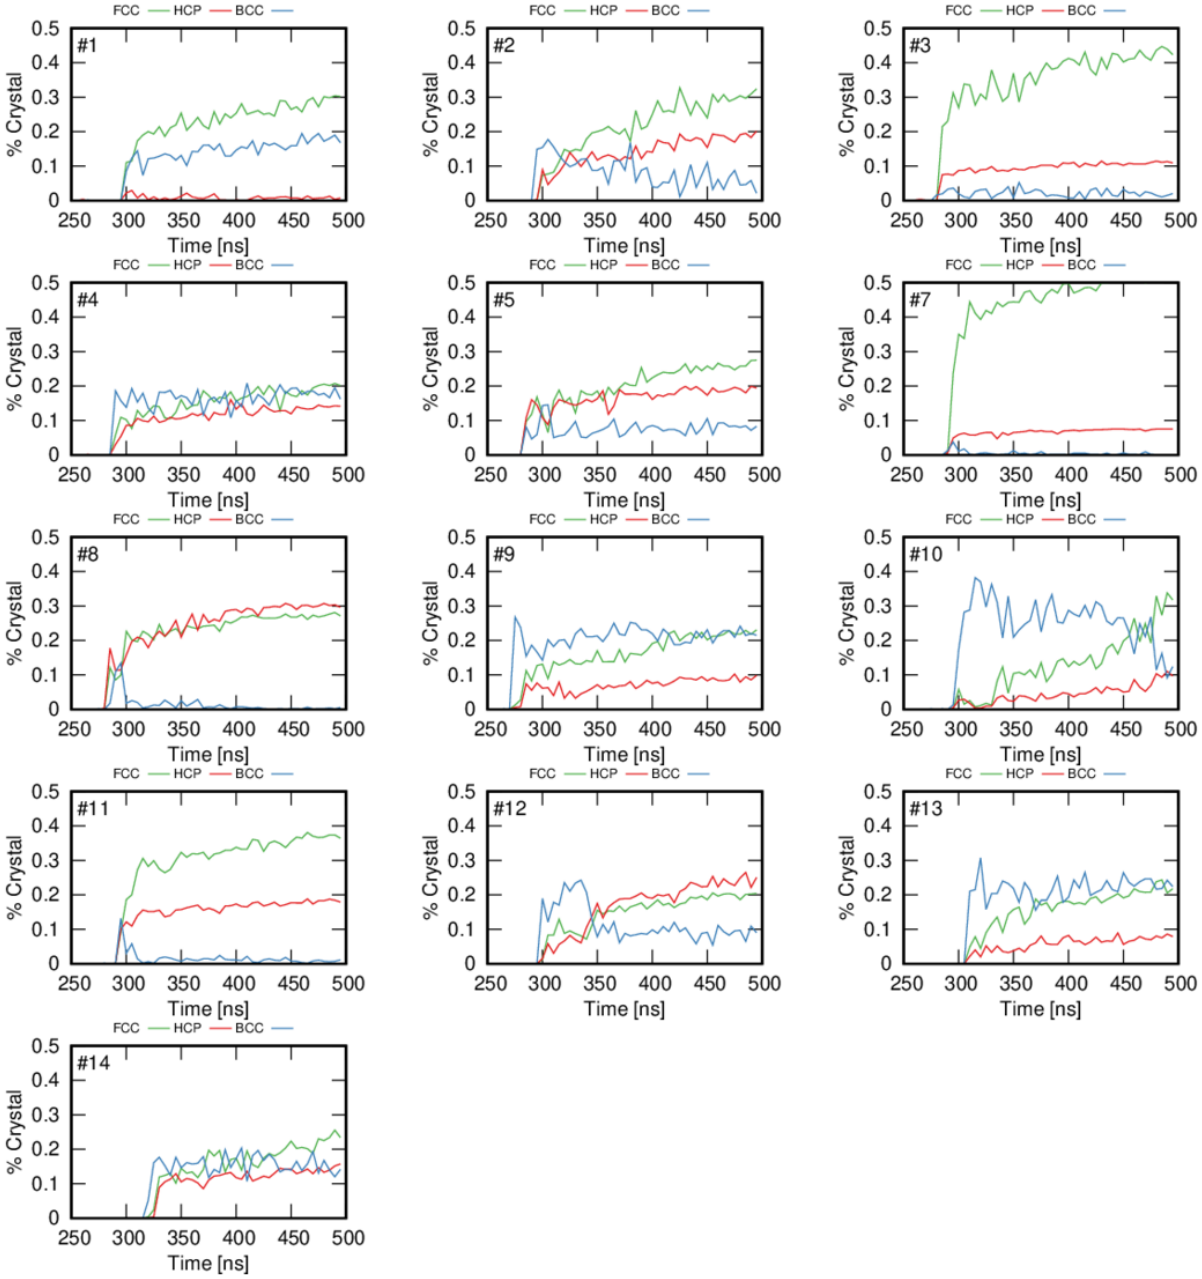


Figure S3: Crystallization kinetics of $Ni_3Al$ nanocrystals at $\tau$ = 200 ns.

**BCC peak**

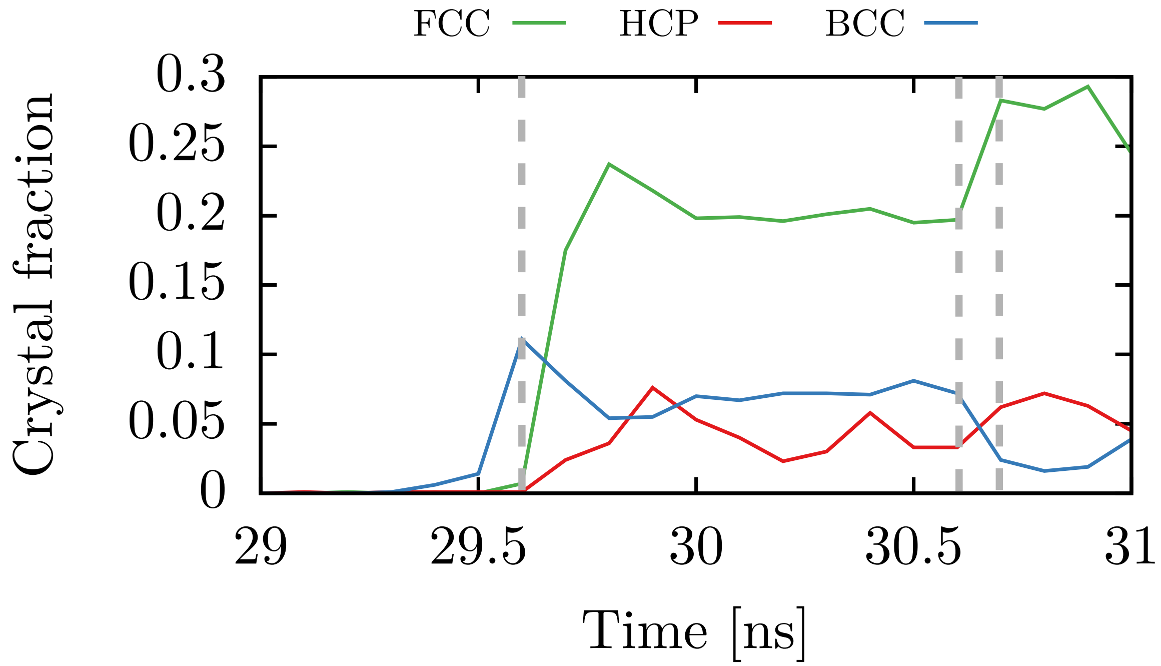


Figure S4: Temporal evolution of the crystal fraction with a quench duration equal to 50 ns as shown in Fig.2 of the main text but focused on the short time scales.

## Metadynamics simulations

Figure S5 shows the temporal evolution of the employed order parameters $S$ and $E$. It appears that several transitions between liquid and crystal and also from crystal to crystal are reversibly sampled, thus suggesting the convergence of the metadynamics simulations.

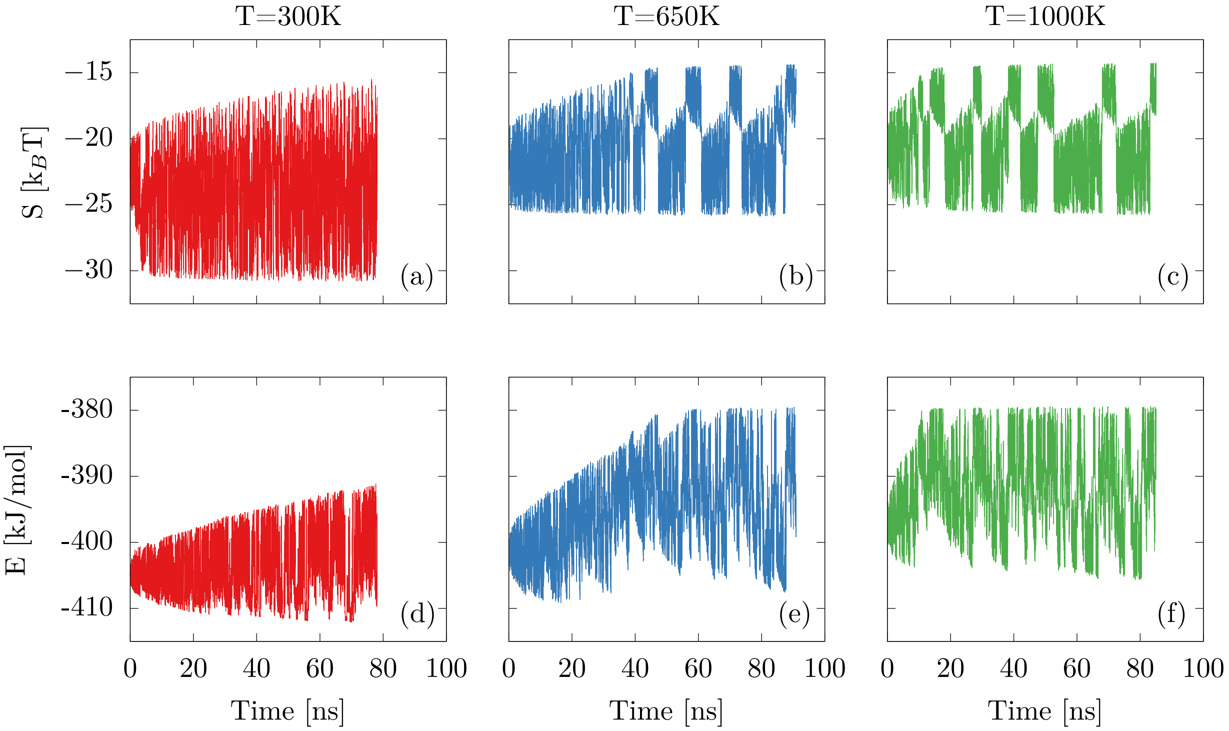


Figure S5: Temporal evolution of the collective variables $S$ and $E$ during the metadynamics calculations for different temperatures.

## Error bars on the free energy landscapes

In the main text free energy landscapes at different temperatures are presented as time averages of the instantaneous bias profiles $V_G(S, E, t)$ over the last half of the simulation. In order to estimate the error bars on the free energy landscapes, we adopt the principle of block averaging and divide the last half of the temporal evolution in $n$ intervals of duration $\tau_n$. A free energy surface is then computed for each interval (indicated with $i$) as time average of $V_G(S, E, t)$:

$$\overline{V_G^i}(S, E) = \frac{1}{\tau_n} \int_{i\tau_n}^{(i+1)\tau_n} V_G(S, E, t)\, dt \tag{S.1}$$

The following analysis is restricted to the region of lowest free energy ($F < 150 k_B T$) in $(S, E)$ space. As discussed in Ref.,[S1,S2] after an initial transient time the free-energy wells are filled by the bias potential: in favorable conditions (mainly related to a good choice of the collective variables) the dynamics becomes stationary, with a flat probability histogram. Therefore, if the duration $\tau_n$ is long enough (longer than their correlation time), the profiles are uncorrelated and random and belong to a same distribution, the standard error of the mean free energy profile is then the standard deviation of the $n$ profiles $\overline{V_G^i}$ (after setting to zero the average value of each surface) divided by $\sqrt{n}$.

From Fig. S6, it appears that using $n < 8$, the average error bars for $T = 1000K$, $T = 650K$ and $T = 300K$ are around respectively $10k_BT$, $5k_BT$ and $10k_BT$. Finally, Fig. S7 shows a similar mapping of the error bar for two different values of $n$.

# References


(S1) Crespo, Y.; Marinelli, F.; Pietrucci, F.; Laio, A. Metadynamics convergence law in a multidimensional system. *Phys. Rev. E* **2010**, *81*, 055701.

(S2) Bussi, G.; Laio, A. Using metadynamics to explore complex free-energy landscapes. *Nat. Rev. Phys.* **2020**, 1–13.

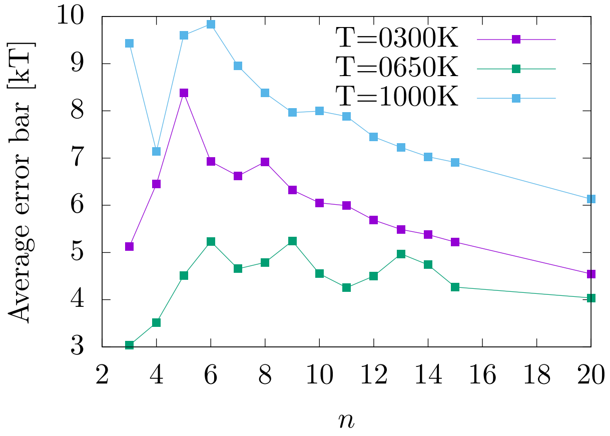


Figure S6: Average error bar as a function of the number of intervals $n$ for the investigated temperatures.

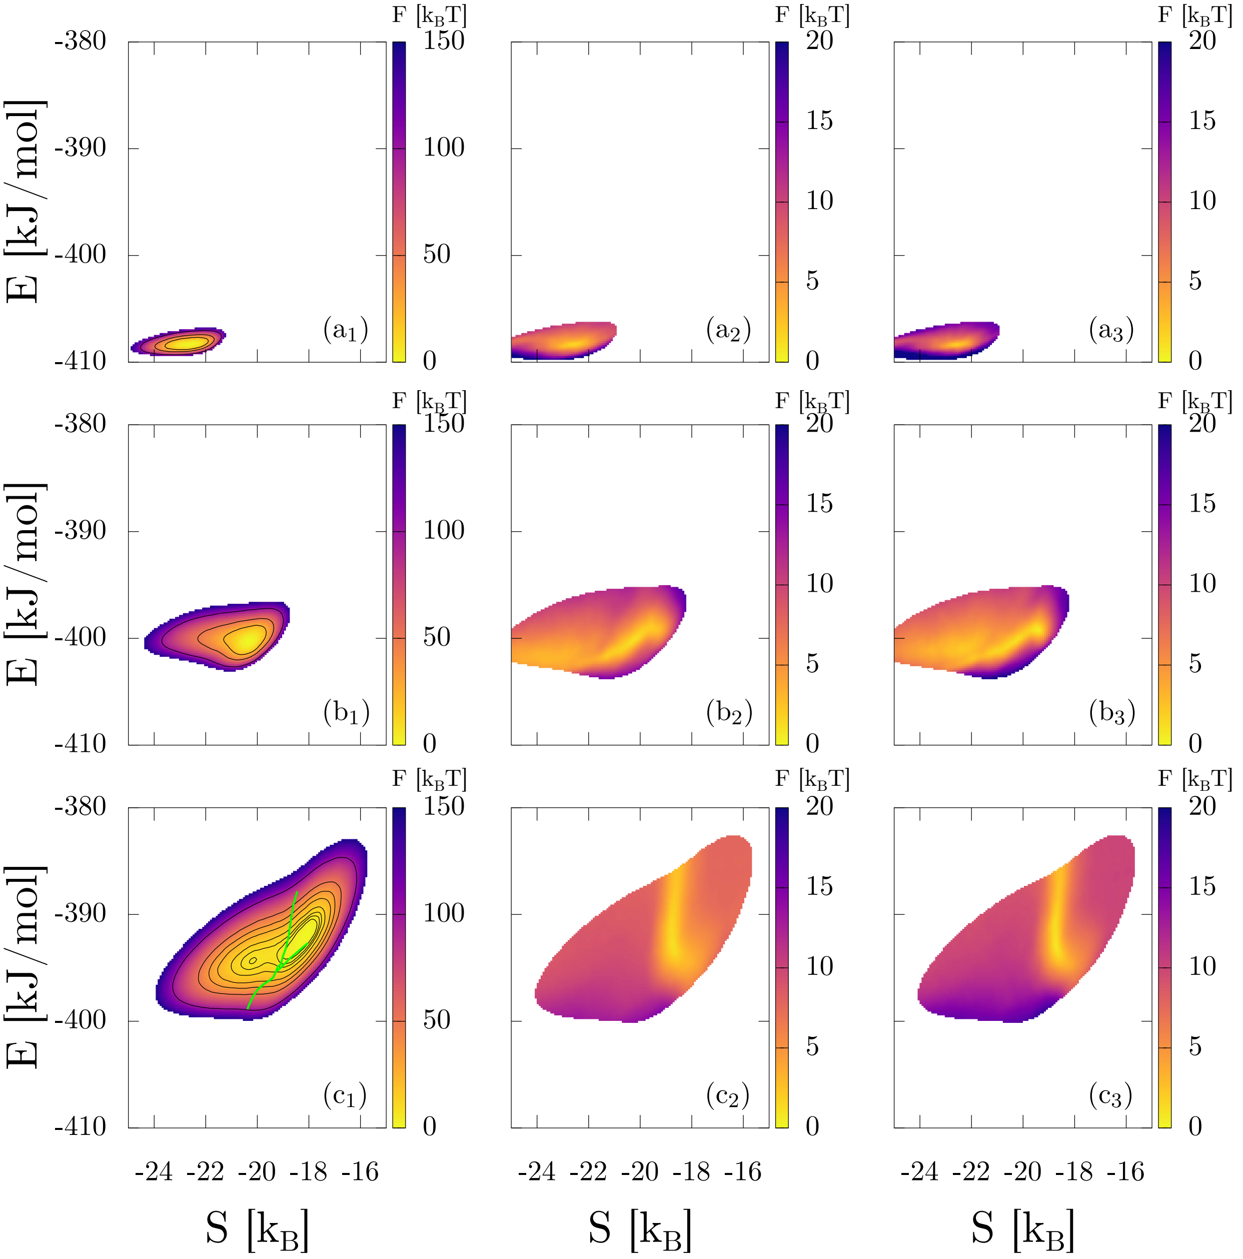


Figure S7: Error bar estimation for the three investigated temperatures $T = 300$K (a), $T = 650$K (b) and $T = 1000$K (c). The first column correspond to the original free energy landscape obtained with the last half of the simulation. The second and third column correspond to the corresponding standard error as computed with the last half of the simulation using respectively $n = 10$ and $n = 5$.
